# Supplementary material for: MeTeoR: Practical Reasoning in Datalog with Metric Temporal Operators
Source: arXiv:2201.04596 source file (2022-01-12)
Supplement: Supplementary file 1 [file appendix.tex]

% \section{Appendix 1.1}
\begin{table*}[htb]
  \begin{tabular}{ll}
     \hline
      \textbf{$\Prog$} & \\
      \hline
     \textbf{Manually constructed rules with MTL operators} & \\
     \hline

       \multicolumn{2}{l}{$ResearchAssistantCandidate(x) \gets \boxminus_{[0,5]}UndergraduateStudent(x)$}\\

       \multicolumn{2}{l}{$ResearchAssistantCandidate(x) \gets \diamondminus_{[0,2]}GraduateStudent(x)$}\\

       \multicolumn{2}{l}{$ResearchAssistantCandidate(x) \gets \boxplus_{[0,2]}TeachingAssistant(x)$}\\

       \multicolumn{2}{l}{$ResearchAssistant(x) \gets undergraduateDegreeFrom(x,y), \boxminus_{[0,3]}ResearchAssistantCandidate(x)$}\\

       \multicolumn{2}{l}{$ResearchAssistant(x) \gets mastersDegreeFrom(x,y), \boxminus_{[0,1]}ResearchAssistantCandidate(x)$}\\

       \multicolumn{2}{l}{$LecturerCandidate(x) \gets \boxminus_{[0,2]}ResearchAssistant(x)$}\\

       \multicolumn{2}{l}{$LecturerCandidate(x) \gets \boxminus_{[0,4]}ResearchAssistantCandidate(x)$}\\

       \multicolumn{2}{l}{$LecturerCandidate(x) \gets \boxminus_{[0,1]}GraduateStudent(x),publicationAuthor(y,x)\Si_{(0, 1]}Publication(y)$}\\

      \multicolumn{2}{l}{$Lecturer(x)  \gets LecturerCandidate(x)\Ui_{(0, 2]}researchInterest(x,y)$} \\

        \multicolumn{2}{l}{$Lecturer(x)  \gets \boxplus_{[1,5]}LecturerCandidate(x)$} \\

        \multicolumn{2}{l}{$AssistantProfessorCandidate(x) \gets \diamondminus_{[1,3]}Lecturer(x)$}\\

       \multicolumn{2}{l}{$AssistantProfessorCandidate(x) \gets \boxminus_{[1,2]}LecturerCandidate(x), \diamondplus_{[0,3]}publicationAuthor(z,x)$}\\

       \multicolumn{2}{l}{$AssistantProfessorCandidate(x) \gets \boxminus_{[1,2]}LecturerCandidate(x), \diamondminus_{[0,3]}doctoralDegreeFrom(x,y)$}\\

       \multicolumn{2}{l}{$AssociateProfessorCandidate(x) \gets \boxminus_{[1,3]}Lectuer(x), \diamondminus_{[0,3]}doctoralDegreeFrom(x,y), publicationAuthor(y,x)$}\\

       \multicolumn{2}{l}{$AssociateProfessorCandidate(x) \gets \boxminus_{[1,5]}AssistantProfessorCandidate(x)$}\\

       \multicolumn{2}{l}{$AssociateProfessorCandidate(x) \gets \boxminus_{[1,3]}AssistantProfessor(x)$}\\

       \multicolumn{2}{l}{$AssociateProfessorCandidate(x) \gets \boxminus_{[1,2]}AssistantProfessorCandidate(x), doctoralDegreeFrom(x,y)$}\\

      \multicolumn{2}{l}{$AssociateProfessor(x) \gets \diamondminus_{[1,2]}AssociateProfessorCandidate(x))$}\\

      \multicolumn{2}{l}{$AssociateProfessorCandidate(x) \gets \boxplus_{[1,3]}AssistantProfessor(x)$}\\

      \multicolumn{2}{l}{$FullProfessorCandidate(x) \gets \boxplus_{[1,2]}AssociateProfessorCandidate(x), \diamondminus_{[0, 3]}publicationAuthor(y,x)$}\\

      \multicolumn{2}{l}{$FullProfessorCandidate(x) \gets \boxminus_{[1,2]}AssociateProfessor(x), \diamondminus_{[0,3]}publicationAuthor(y,x)$}\\

     \multicolumn{2}{l}{$GoodDepartment(y)  \gets  \boxminus_{[0,2]}worksFor(x,y),FullProfessor(x)$} \\
     \multicolumn{2}{l}{$SmartStudent(x)  \gets  UndergraduateStudent(x), \diamondplus_{[1,2]}memberOf(x,y), GoodDepartment(y)$}\\
     \multicolumn{2}{l}{$SmartStudent(x)  \gets GraduateStudent(x), \diamondplus_{[1,3]}memberOf(x,y), GoodDepartment(y)$}\\
     \multicolumn{2}{l}{$GoodDepartment(x)  \gets \boxplus_{[0,2]}SmartStudent(x), \diamondminus_{[0,1]}publicationAuthor(y,x)$}\\

      \multicolumn{2}{l}{$ScientistCandidate(x)
      \gets Diamondminus[0,5]a1:doctoralDegreeFrom(x,y)$} \\

      \multicolumn{2}{l}{$Scientist(x) \gets Boxminus[0,4]ScientistCandidate(x)$}\\

     \multicolumn{2}{l}{$Scientist(x) \gets \diamondminus_{[1,2]}FullProfessor(x)$} \\
     \multicolumn{2}{l}{$FullProfessor(x)  \gets  \diamondminus_{[1,2]}Scientist(x)$} \\

     \hline
     \textbf{LUBM original rules} & \\
     \hline
     University(x1)$\gets$ mastersDegreeFrom(x,x1)
     &degreeFrom(x,y)$\gets$ hasAlumnus(y,x)\\
     hasAlumnus(x,y)$\gets$ degreeFrom(y,x)
     &Employee(x)$\gets$ Faculty(x)\\
     Faculty(x)$\gets$ Professor(x)
     &Professor(x)$\gets$ AssociateProfessor(x)\\
     Person(x1)$\gets$ member(x,x1)
     &Professor(x)$\gets$ AssistantProfessor(x)\\
     Professor(x)$\gets$ Chair(x)
     &worksFor(x,y)$\gets$ headOf(x,y)\\
     Person(x)$\gets$ degreeFrom(x,x1)
     &University(x1)$\gets$ degreeFrom(x,x1)\\
     Person(x1)$\gets$ hasAlumnus(x,x1)
     &memberOf(x,y)$\gets$ member(y,x)\\
     member(x,y)$\gets$ memberOf(y,x)
     &Course(x1)$\gets$ teacherOf(x,x1)\\
     University(x)$\gets$ hasAlumnus(x,x1)
     &Person(x)$\gets$ telephone(x,x1)\\
     Organization(x1)$\gets$ subOrganizationOf(x,x1)
     &memberOf(x,y)$\gets$ worksFor(x,y)\\
     Person(x)$\gets$ Employee(x)
     &Person(x)$\gets$ advisor(x,x1)\\
     Organization(x)$\gets$ member(x,x1)
     &Organization(x)$\gets$ Department(x)\\
     Faculty(x)$\gets$ Lecturer(x)
     &Person(x1)$\gets$ publicationAuthor(x,x1)\\
     Professor(x1)$\gets$ advisor(x,x1)
     &Work(x)$\gets$ Course(x)\\
     Professor(x)$\gets$ FullProfessor(x)
     &degreeFrom(x,y)$\gets$ doctoralDegreeFrom(x,y)\\
     TeachingAssistant(x)$\gets$ teachingAssistantOf(x,x1)
     &Person(x)$\gets$ undergraduateDegreeFrom(x,x1)\\
     Organization(x)$\gets$ University(x)
     &Person(x)$\gets$ doctoralDegreeFrom(x,x1)\\
     University(x1)$\gets$ doctoralDegreeFrom(x,x1)
     &Course(x1)$\gets$ teachingAssistantOf(x,x1)\\
     University(x1)$\gets$ undergraduateDegreeFrom(x,x1)
     &degreeFrom(x,y)$\gets$ mastersDegreeFrom(x,y)\\
     Person(x)$\gets$ GraduateStudent(x)
     &Person(x)$\gets$ ResearchAssistant(x)\\
     Student(x)$\gets$ UndergraduateStudent(x)
     &degreeFrom(x,y)$\gets$ undergraduateDegreeFrom(x,y)\\
     Publication(x)$\gets$ publicationAuthor(x,x1)
     &Person(x)$\gets$ mastersDegreeFrom(x,x1)\\
     Organization(x)$\gets$ ResearchGroup(x)
     &Faculty(x)$\gets$ teacherOf(x,x1)\\
     Person(x)$\gets$ Chair(x)
     &Course(x)$\gets$ GraduateCourse(x)\\
     Person(x)$\gets$ TeachingAssistant(x)
     &Person(x)$\gets$ Student(x)\\
     Person(x)$\gets$ emailAddress(x,x1)
     &Chair(x)$\gets$ Person(x), headOf(x,x1), Department(x1)\\
     Employee(x)$\gets$a1:Person(x), worksFor(x,x1), Organization(x1)
     & Student(x)$\gets$ Person(x), takesCourse(x,x1), Course(x1)\\
     TeachingAssistant(x)$\gets$ Person(x), teachingAssistantOf(x,x1) Course(x1) & \\
     Organization(x)$\gets$ subOrganizationOf(x,y), Person(x), Student(x) & \\
     \hline

  \end{tabular}

\caption{The complete program $\Prog$ including the orignal LUBM rules and $20$ new constructed rules with MTL operators}
\end{table*}

\begin{table}
    \begin{tabular}{ll}
      \hline
      \hline
      \multicolumn{2}{l}{\textbf{$\Prog^1$}}\\
      \hline
      \multicolumn{2}{l}{$ResearchAssistantCandidate(x) \gets \boxminus_{[0,5]}UndergraduateStudent(x)$}\\

      \multicolumn{2}{l}{$ResearchAssistantCandidate(x) \gets \diamondminus_{[0,2]}GraduateStudent(x)$}\\

      \multicolumn{2}{l}{$ResearchAssistantCandidate(x) \gets \boxplus_{[0,2]}TeachingAssistant(x)$}\\

      \multicolumn{2}{l}{$ResearchAssistant(x) \gets undergraduateDegreeFrom(x,y), \boxminus_{[0,3]}ResearchAssistantCandidate(x)$}\\

      \multicolumn{2}{l}{$ResearchAssistant(x) \gets mastersDegreeFrom(x,y), \boxminus_{[0,1]}ResearchAssistantCandidate(x)$}\\

      \hline
      \textbf{$\Prog^2$} \\
      \hline
      \multicolumn{2}{l}{$ResearchAssistantCandidate(x) \gets \boxminus_{[0,5]}UndergraduateStudent(x)$}\\

      \multicolumn{2}{l}{$ResearchAssistantCandidate(x) \gets \diamondminus_{[0,2]}GraduateStudent(x)$}\\

      \multicolumn{2}{l}{$ResearchAssistantCandidate(x) \gets \boxplus_{[0,2]}TeachingAssistant(x)$}\\

      \multicolumn{2}{l}{$ResearchAssistant(x) \gets undergraduateDegreeFrom(x,y), \boxminus_{[0,3]}ResearchAssistantCandidate(x)$}\\

      \multicolumn{2}{l}{$ResearchAssistant(x) \gets mastersDegreeFrom(x,y), \boxminus_{[0,1]}ResearchAssistantCandidate(x)$}\\

      \multicolumn{2}{l}{$LecturerCandidate(x) \gets \boxminus_{[0,2]}ResearchAssistant(x)$}\\

      \multicolumn{2}{l}{$LecturerCandidate(x) \gets \boxminus_{[0,4]}ResearchAssistantCandidate(x)$}\\

      \multicolumn{2}{l}{$LecturerCandidate(x) \gets \boxminus_{[0,1]}GraduateStudent(x),publicationAuthor(y,x)\Si_{(0, 1]}Publication(y)$}\\

     \multicolumn{2}{l}{$Lecturer(x)  \gets LecturerCandidate(x)\Ui_{(0, 2]}researchInterest(x,y)$} \\

       \multicolumn{2}{l}{$Lecturer(x)  \gets \boxplus_{[1,5]}LecturerCandidate(x)$} \\

      \hline
      \textbf{$\Prog^3$} \\
      \hline

      \multicolumn{2}{l}{$ResearchAssistantCandidate(x) \gets \boxminus_{[0,5]}UndergraduateStudent(x)$}\\

      \multicolumn{2}{l}{$ResearchAssistantCandidate(x) \gets \diamondminus_{[0,2]}GraduateStudent(x)$}\\

      \multicolumn{2}{l}{$ResearchAssistantCandidate(x) \gets \boxplus_{[0,2]}TeachingAssistant(x)$}\\

      \multicolumn{2}{l}{$ResearchAssistant(x) \gets undergraduateDegreeFrom(x,y), \boxminus_{[0,3]}ResearchAssistantCandidate(x)$}\\

      \multicolumn{2}{l}{$ResearchAssistant(x) \gets mastersDegreeFrom(x,y), \boxminus_{[0,1]}ResearchAssistantCandidate(x)$}\\

      \multicolumn{2}{l}{$LecturerCandidate(x) \gets \boxminus_{[0,2]}ResearchAssistant(x)$}\\

      \multicolumn{2}{l}{$LecturerCandidate(x) \gets \boxminus_{[0,4]}ResearchAssistantCandidate(x)$}\\

      \multicolumn{2}{l}{$LecturerCandidate(x) \gets \boxminus_{[0,1]}GraduateStudent(x),publicationAuthor(y,x)\Si_{(0, 1]}Publication(y)$}\\

     \multicolumn{2}{l}{$Lecturer(x)  \gets LecturerCandidate(x)\Ui_{(0, 2]}researchInterest(x,y)$} \\

       \multicolumn{2}{l}{$Lecturer(x)  \gets \boxplus_{[1,5]}LecturerCandidate(x)$} \\

       \multicolumn{2}{l}{$AssistantProfessorCandidate(x) \gets \diamondminus_{[1,3]}Lecturer(x)$}\\

      \multicolumn{2}{l}{$AssistantProfessorCandidate(x) \gets \boxminus_{[1,2]}LecturerCandidate(x), \diamondplus_{[0,3]}publicationAuthor(z,x)$}\\

      \multicolumn{2}{l}{$AssistantProfessorCandidate(x) \gets \boxminus_{[1,2]}LecturerCandidate(x), \diamondminus_{[0,3]}doctoralDegreeFrom(x,y)$}\\

      \multicolumn{2}{l}{$AssociateProfessorCandidate(x) \gets \boxminus_{[1,3]}Lectuer(x), \diamondminus_{[0,3]}doctoralDegreeFrom(x,y), publicationAuthor(y,x)$}\\

      \multicolumn{2}{l}{$AssociateProfessorCandidate(x) \gets \boxminus_{[1,5]}AssistantProfessorCandidate(x)$}\\

      \multicolumn{2}{l}{$AssociateProfessorCandidate(x) \gets \boxminus_{[1,3]}AssistantProfessor(x)$}\\

      \multicolumn{2}{l}{$AssociateProfessorCandidate(x) \gets \boxminus_{[1,2]}AssistantProfessorCandidate(x), doctoralDegreeFrom(x,y)$}\\

     \multicolumn{2}{l}{$AssociateProfessor(x) \gets \diamondminus_{[1,2]}AssociateProfessorCandidate(x))$}\\

     \multicolumn{2}{l}{$AssociateProfessorCandidate(x) \gets \boxplus_{[1,3]}AssistantProfessor(x)$}\\

     \multicolumn{2}{l}{$FullProfessorCandidate(x) \gets \boxplus_{[1,2]}AssociateProfessorCandidate(x), \diamondminus_{[0, 3]}publicationAuthor(y,x)$}\\

     \multicolumn{2}{l}{$FullProfessorCandidate(x) \gets \boxminus_{[1,2]}AssociateProfessor(x), \diamondminus_{[0,3]}publicationAuthor(y,x)$}\\

      \hline
    \end{tabular}
    \caption{Three sub programs $\Prog^1$, $\Prog^2$, $\Prog^3$ used in our experiments}
\end{table}

\begin{table}
  \begin{tabular}{l|l}
    \hline
    \multirow{10}{*}{T1} &UndergraduateStudent(http://www.department9.university9.edu/undergraduatestudent471)@(13.0,20.0]\\
  &TeachingAssistant(http://www.department9.university9.edu/graduatestudent38)@[19.5,19.5]\\
  &Course(http://www.department9.university9.edu/course36)@[8.5,13.0]\\
  &GraduateStudent(http://www.department9.university4.edu/graduatestudent64)@(7.0,11.0]\\
  &ResearchAssistant(http://www.department9.university1.edu/graduatestudent4)@[18.5,19.5)\\
  &GraduateCourse(http://www.department9.university9.edu/graduatecourse33)@[0.0,14.0]\\
  &AssociateProfessor(http://www.department9.university9.edu/associateprofessor10)@(5.5,7.5]\\
  &ResearchGroup(http://www.department9.university11.edu/researchgroup2)@(16.5,18.0]\\
  &AssistantProfessor(http://www.department9.university9.edu/assistantprofessor0)@[11.5,20.0]\\
  &FullProfessor(http://www.department9.university5.edu/fullprofessor7)@(19.5,20.0]\\
  \hline

  \multirow{10}{*}{T2} & FullProfessorCandidate(http://www.department9.university9.edu/associateprofessor10)@(5.5,7.5]\\
&AssociateProfessorCandidate(http://www.department9.university8.edu/associateprofessor3)@[25.0,25.0]\\
&AssociateProfessorCandidate(http://www.department9.university9.edu/assistantprofessor0)@[11.5,20.0]\\
&FullProfessorCandidate(http://www.department9.university9.edu/assistantprofessor1)@[0.0,19.5)\\
&AssistantProfessorCandidate(http://www.department9.university9.edu/associateprofessor6)@[4.5,19.5]\\
&AssociateProfessorCandidate(http://www.department9.university2.edu/graduatecourse11)@[11.0,18.0)\\
&LectuerCandidate(http://www.department9.university1.edu/fullprofessor7)@(19.5,20.0]\\
&AssociateProfessorCandidate(http://www.department9.university2.edu/fullprofessor5)@(14.0,16.5)\\
&FullProfessorCandidate(http://www.department9.university3.edu/fullprofessor8)@(2.5,9.5)\\
&FullProfessorCandidate(http://www.department12.university6.edu/fullprofessor8)@(4.5,19.5)\\
\hline

\multirow{10}{*}{T3} & SmartStudent(http://www.department9.university9.edu/undergraduatestudent471)@[13.0,13.0]\\
&SmartStudent(http://www.department9.university9.edu/undergraduatestudent275)@(17.5,18.5]\\
&SmartStudent(http://www.department9.university9.edu/undergraduatestudent507)@(9.5,13.5)\\
&SmartStudent(http://www.department9.university9.edu/undergraduatestudent311)@[1.5,12.5]\\
&SmartStudent(http://www.department9.university9.edu/undergraduatestudent344)@[9.0,16.5)\\
&SmartStudent(http://www.department9.university9.edu/undergraduatestudent133)@[2.5,5.5)\\
&SmartStudent(http://www.department9.university9.edu/undergraduatestudent337)@(7.5,14.0)\\
&GoodDepartment(http://www.department9.university9.edu)@[10.5,20.5)\\
&GoodDepartment(http://www.department0.university0.edu)@[1.0,6.5)\\
&GoodDepartment(http://www.department1.university0.edu)@[2.0,12.5)\\
\hline
\multirow{10}{*}{T4} & Scientist(http://www.department9.university9.edu/fullprofessor7)@(21.5,23.0]\\
&Scientist(http://www.department9.university9.edu/fullprofessor5)@(15.0,20.5)\\
&Scientist(http://www.department9.university9.edu/fullprofessor8)@(2.5,19.5)\\
&FullProfessor(http://www.department9.university9.edu/fullprofessor0)@[11.0,25.0]\\
&FullProfessor(http://www.department9.university9.edu/fullprofessor9)@[2.5,36.5)\\
&FullProfessor(http://www.department9.university9.edu/fullprofessor3)@(4.5,43.0)\\
&Scientist(http://www.department9.university9.edu/fullprofessor6)@[16.5,50.0]\\
&FullProfessor(http://www.department9.university9.edu/fullprofessor2)@(1.0,45.5)\\
&Scientist(http://www.department9.university9.edu/fullprofessor4)@(1.0,19.0]\\
&Scientist(http://www.department9.university9.edu/fullprofessor1)@[11.0,19.5]\\
\hline
\multirow{10}{*}{T5} & FullProfessor(http://www.department9.university9.edu/fullprofessor7)@(1.5,2.0]\\
&FullProfessor(http://www.department9.university9.edu/fullprofessor5)@(2.0,3.5)\\
&Scientist(http://www.department9.university9.edu/fullprofessor8)@(1.5,19.5)\\
&FullProfessor(http://www.department9.university9.edu/fullprofessor0)@[1.0,20.0]\\
&Scientist(http://www.department9.university9.edu/fullprofessor9)@[-1.5,6.5)\\
&FullProfessor(http://www.department9.university9.edu/fullprofessor3)@(0.5,13.0)\\
&FullProfessor(http://www.department9.university9.edu/fullprofessor6)@[6.5,20.0]\\
&FullProfessor(http://www.department9.university9.edu/fullprofessor2)@[0.0,15.5)\\
&Scientist(http://www.department9.university9.edu/fullprofessor4)@[-11.0,13.0]\\
&FullProfessor(http://www.department9.university9.edu/fullprofessor1)@[-3.0,19.5]\\
\hline
  \end{tabular}
  \caption{Details of facts used in Table~\ref{tab:recursive}}
\end{table}
